# Supplementary material for: A quantitative study of NLP approaches to question difficulty estimation
Source: arXiv:2305.10236 source file (2023-05-17)
Supplement: Supplementary file 1 [file appendix_datasets.tex]

\section{Experimental Datasets}\label{app:sec:datasets}

\subsection{\race{}}
%TODO ? something else? Such as stats
The original \textit{RACE} dataset and the \textit{RACE-c} dataset are available at:
\begin{itemize}
\item \url{https://www.cs.cmu.edu/$\sim$glai1/data/race/}, 
\item \url{https://github.com/mrcdata/race-c/}.
\end{itemize}

Figure \ref{fig:diff_distr_race} shows the distribution of questions by difficulty in \race{} in the train and test splits.
The three difficulty levels are unbalanced, with $1$ being by far the most frequent, and the distribution is the same in the two splits. 

\begin{figure}
\centering
\begin{subfigure}{0.40\textwidth}
\centering
\includegraphics[width=\textwidth]{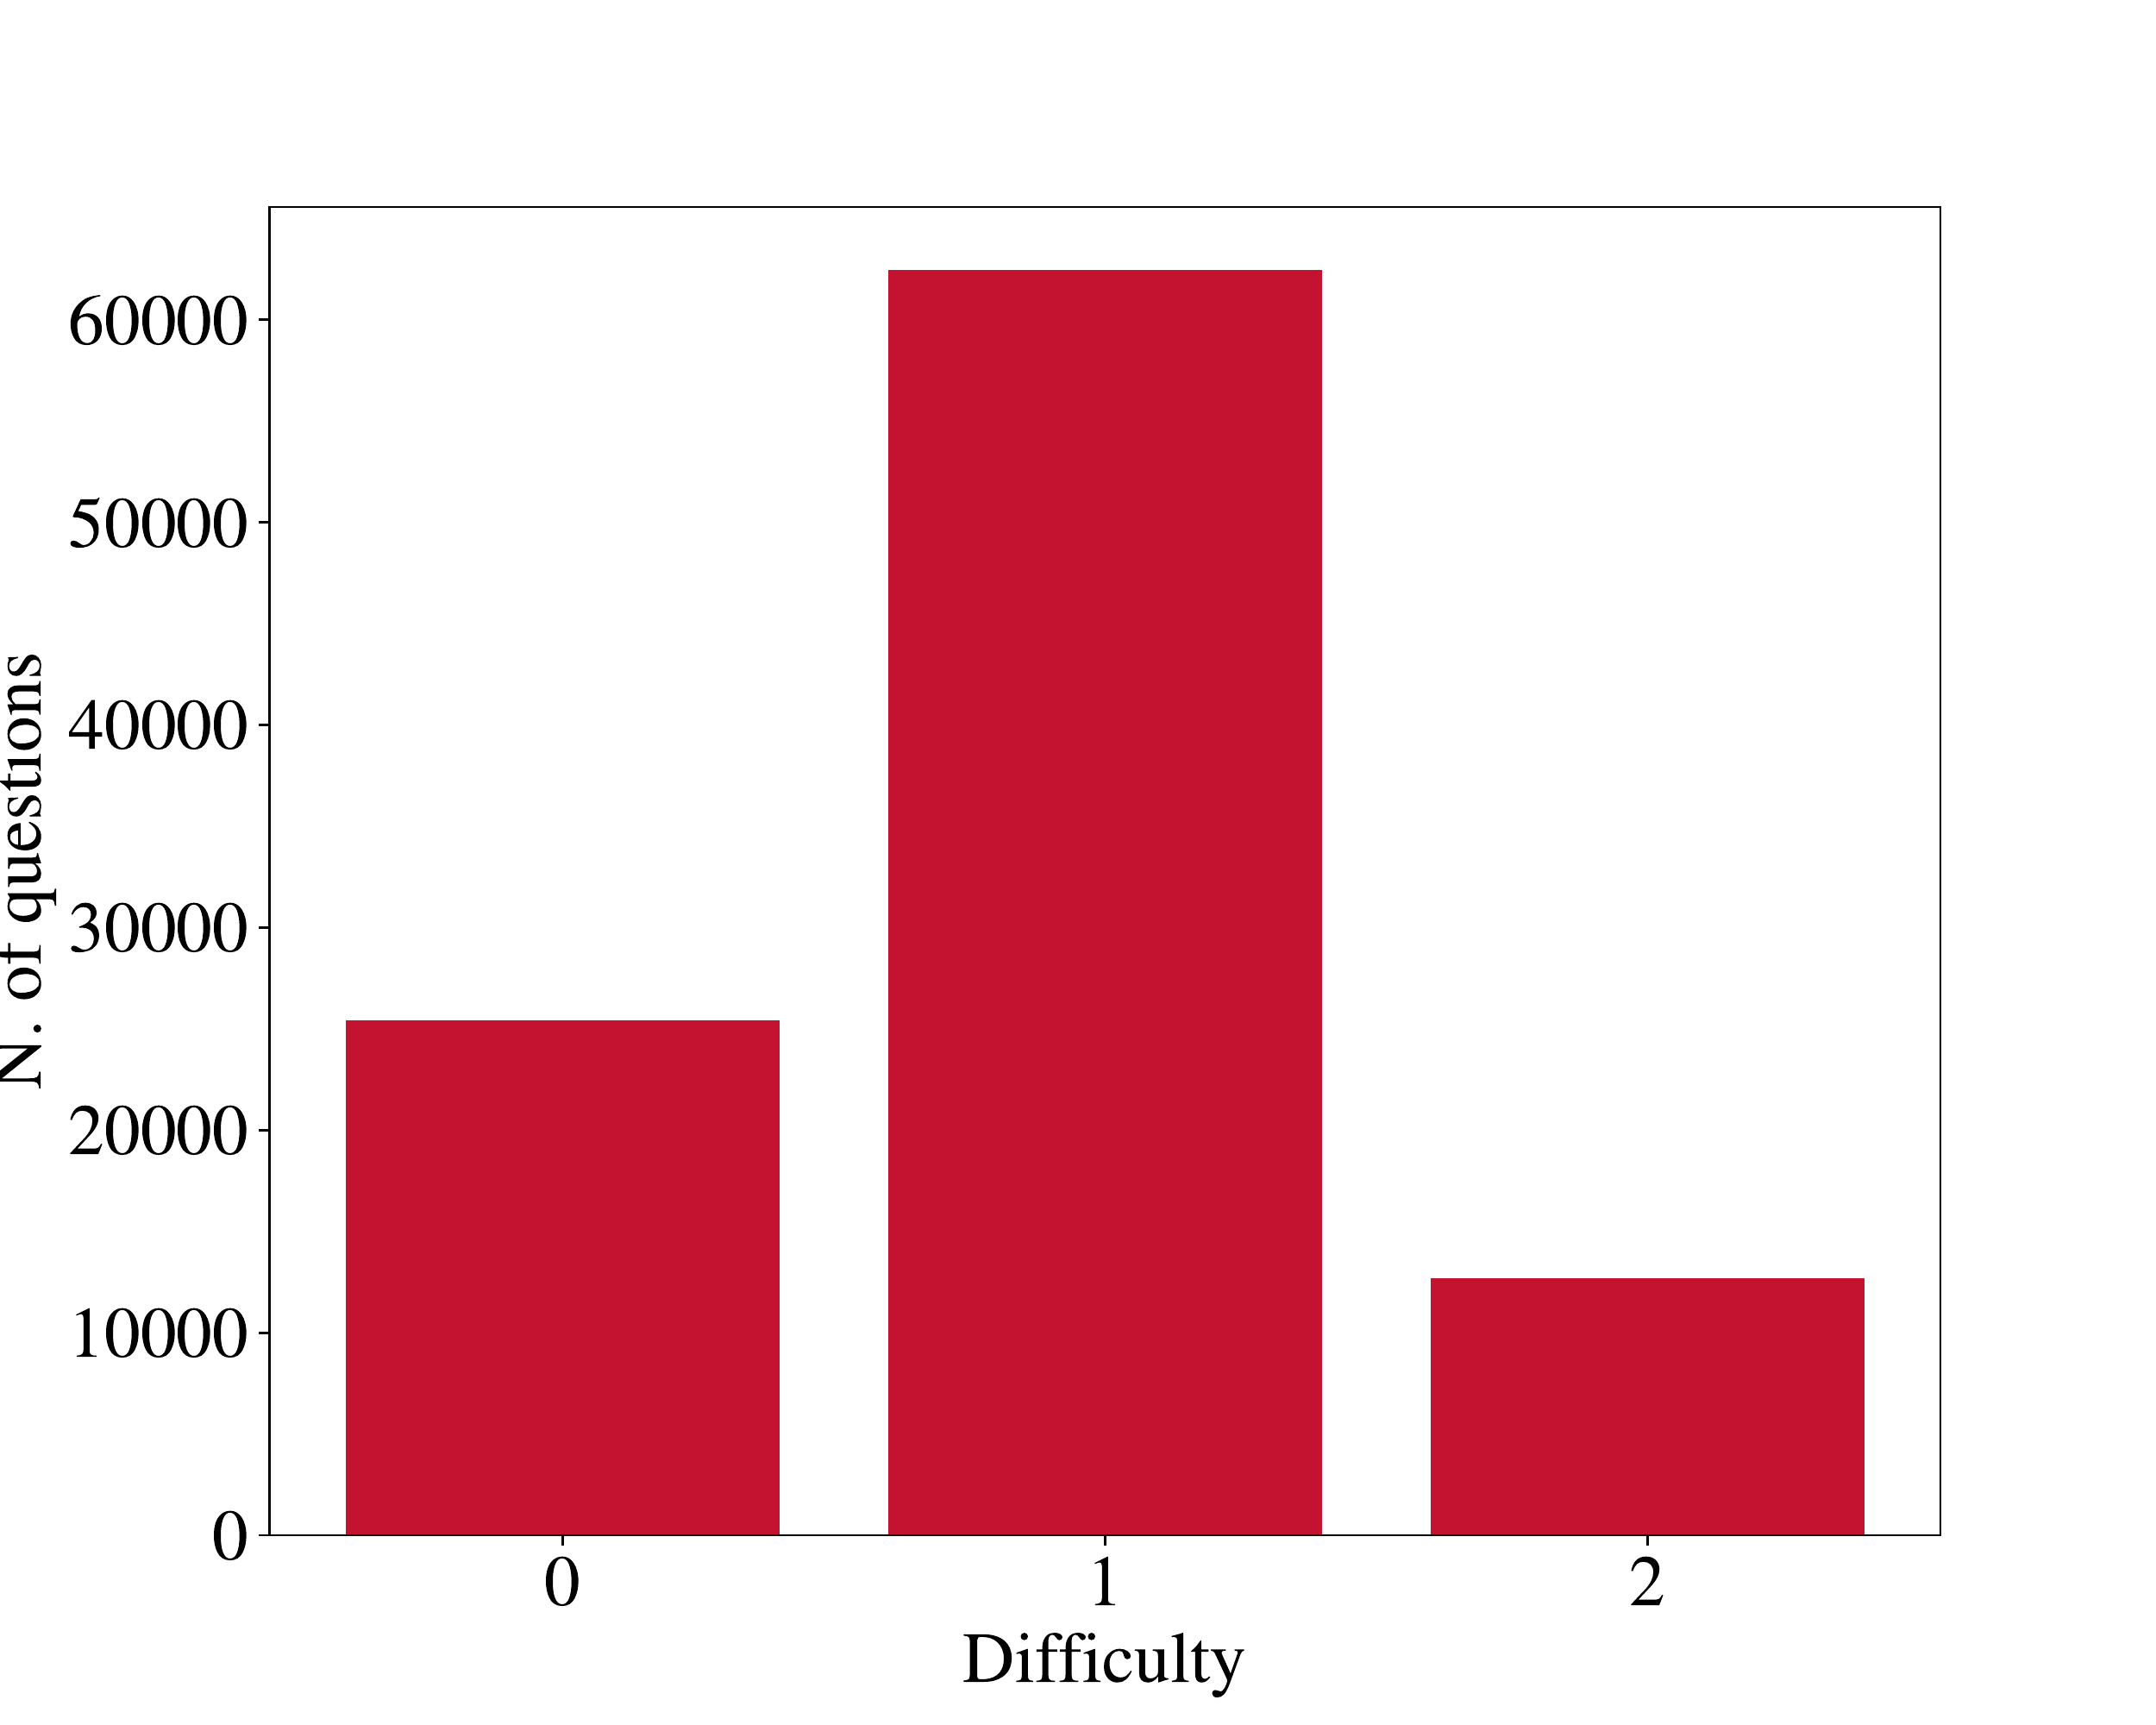}
\caption{Train.}
\label{fig:diff_distr_race_train}
\end{subfigure}
\begin{subfigure}{0.40\textwidth}
\centering
\includegraphics[width=\textwidth]{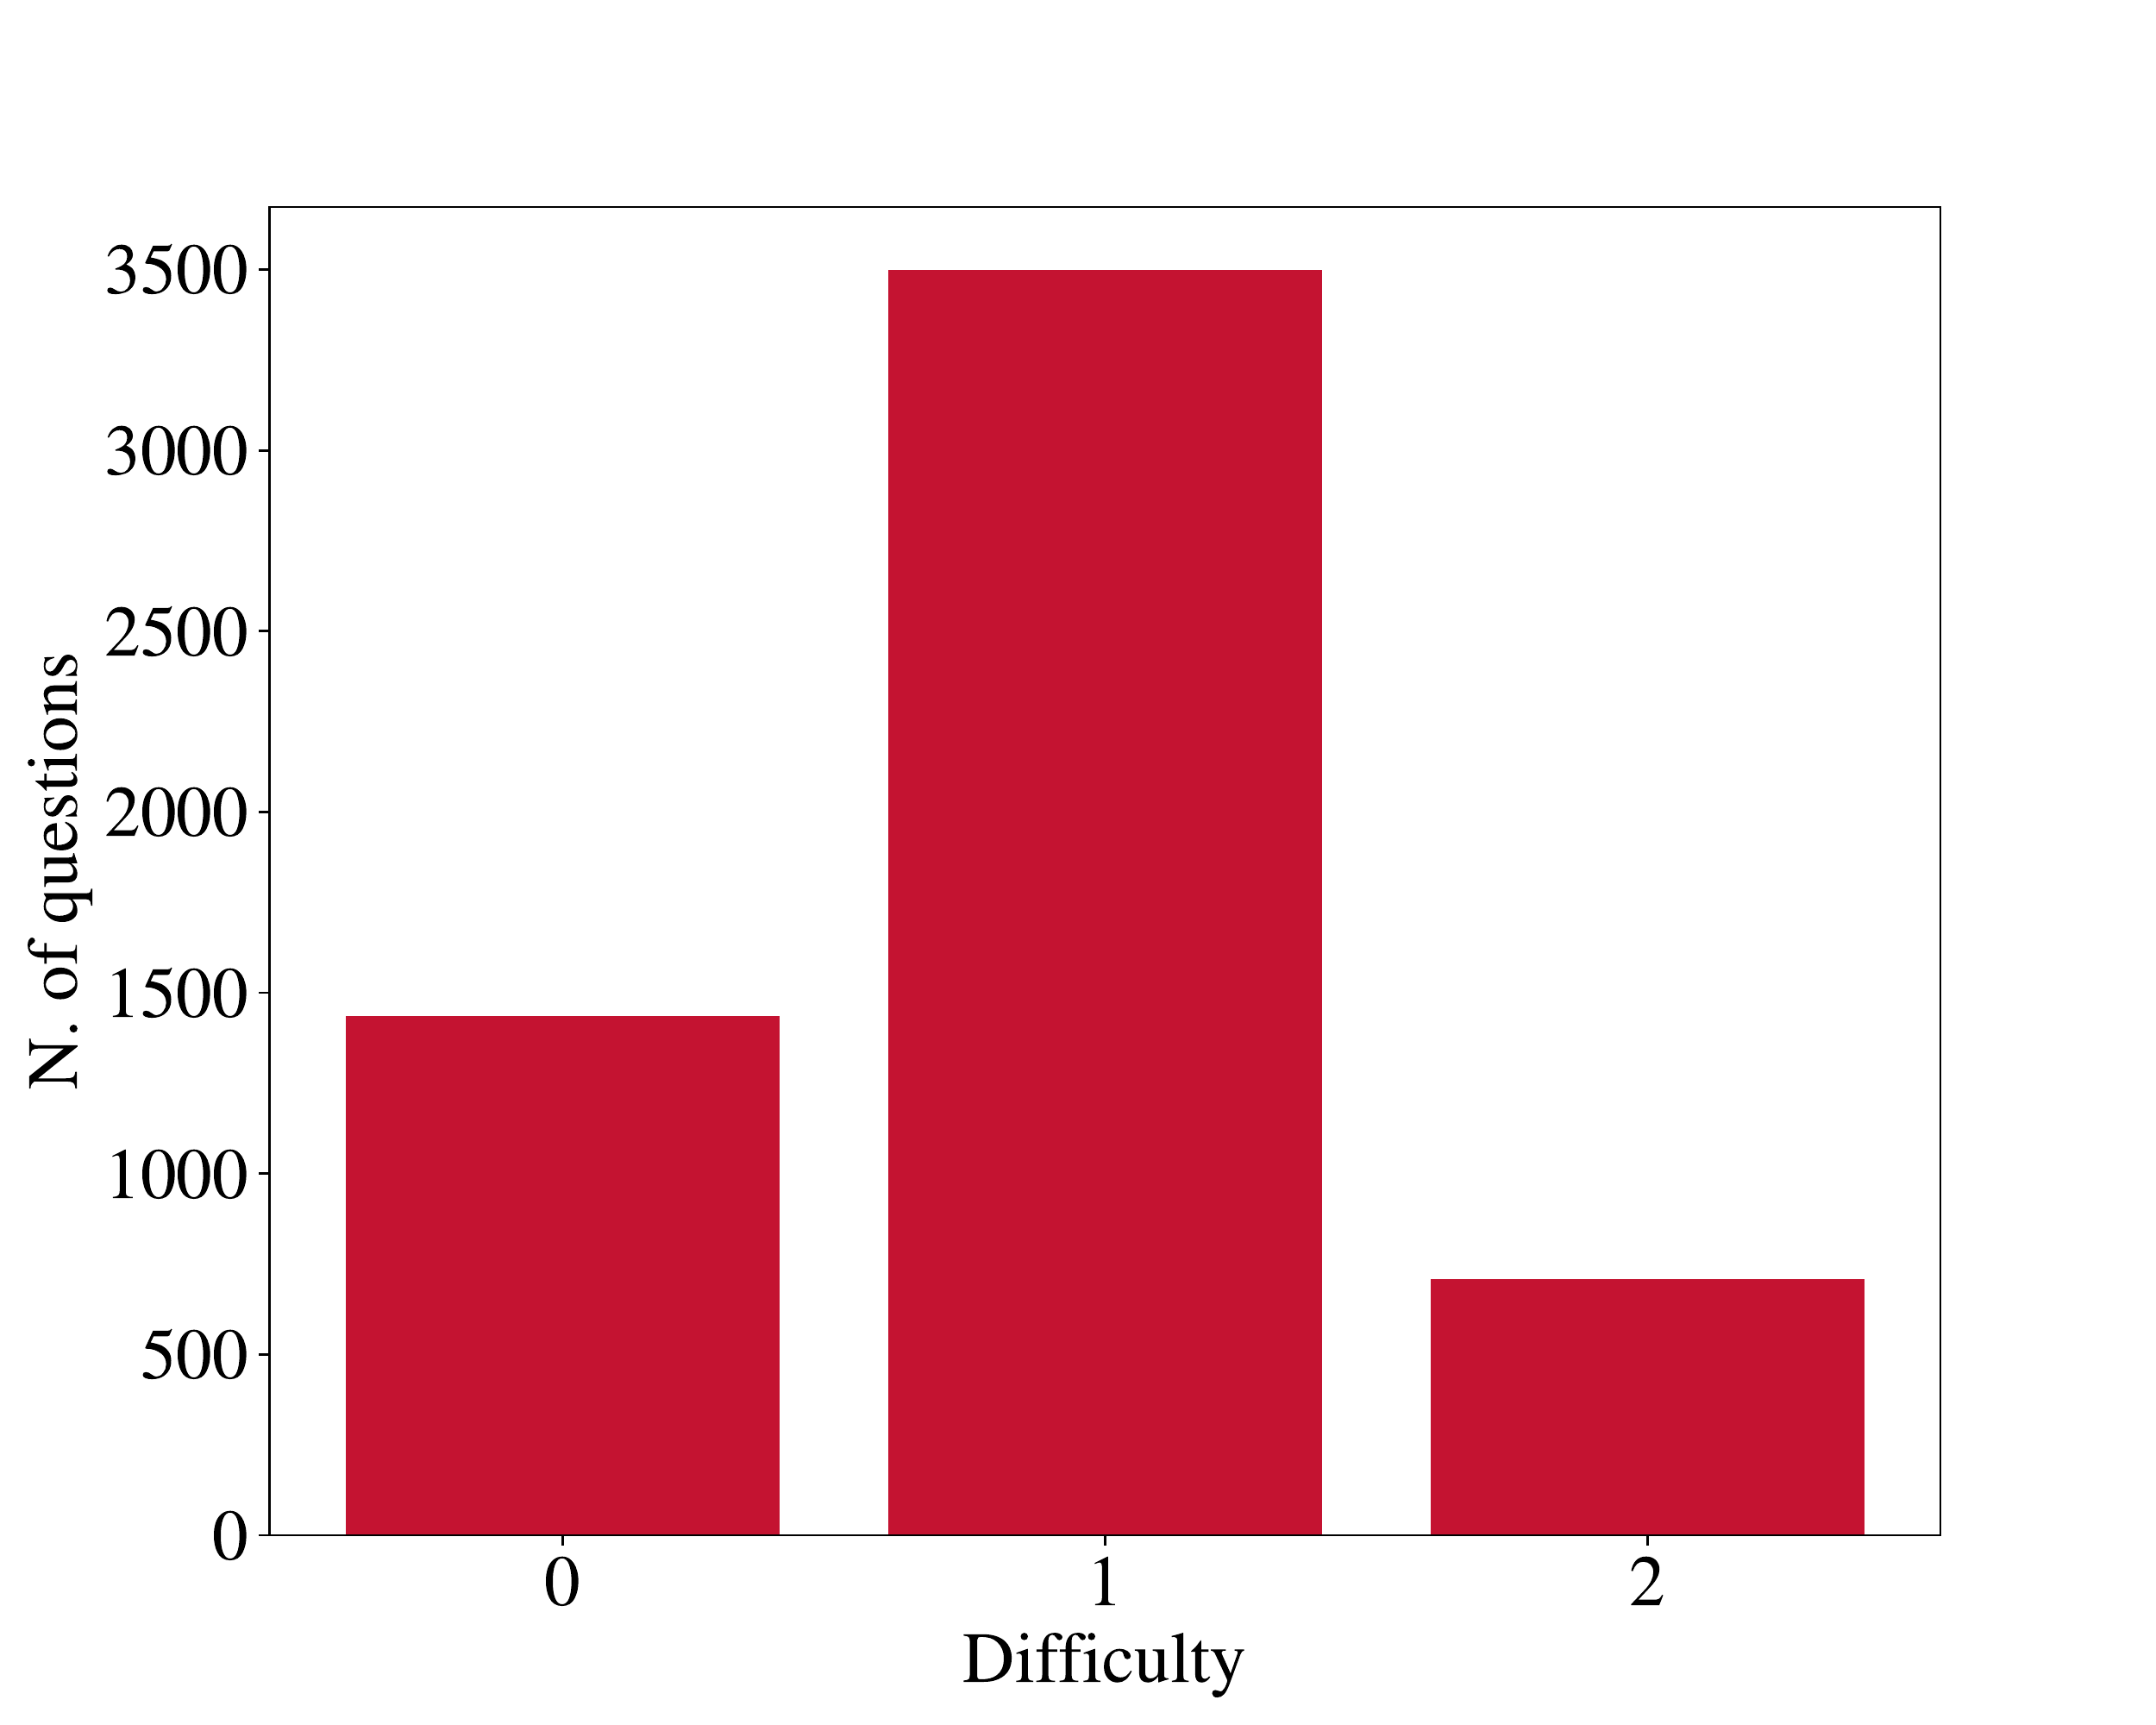}
\caption{Test.}
\label{fig:diff_distr_race_test}
\end{subfigure}
\caption{Question distribution by difficulty in \race{}.}
\label{fig:diff_distr_race}
\end{figure}

\subsection{\arc{}}
%TODO ? something else? Such as stats
\arc{} is available at \url{https://allenai.org/data/arc}.

Figure \ref{fig:diff_distr_arc} shows the distribution of questions by difficulty in \arc{} in the train and test splits (before balancing).
The difficulty levels are very unbalanced, with $8$ being by far the most frequent, and some levels (\eg{} 3 and 6) are a very limited number of questions associated with them.

\begin{figure}
\centering
\begin{subfigure}{0.40\textwidth}
\centering
\includegraphics[width=\textwidth]{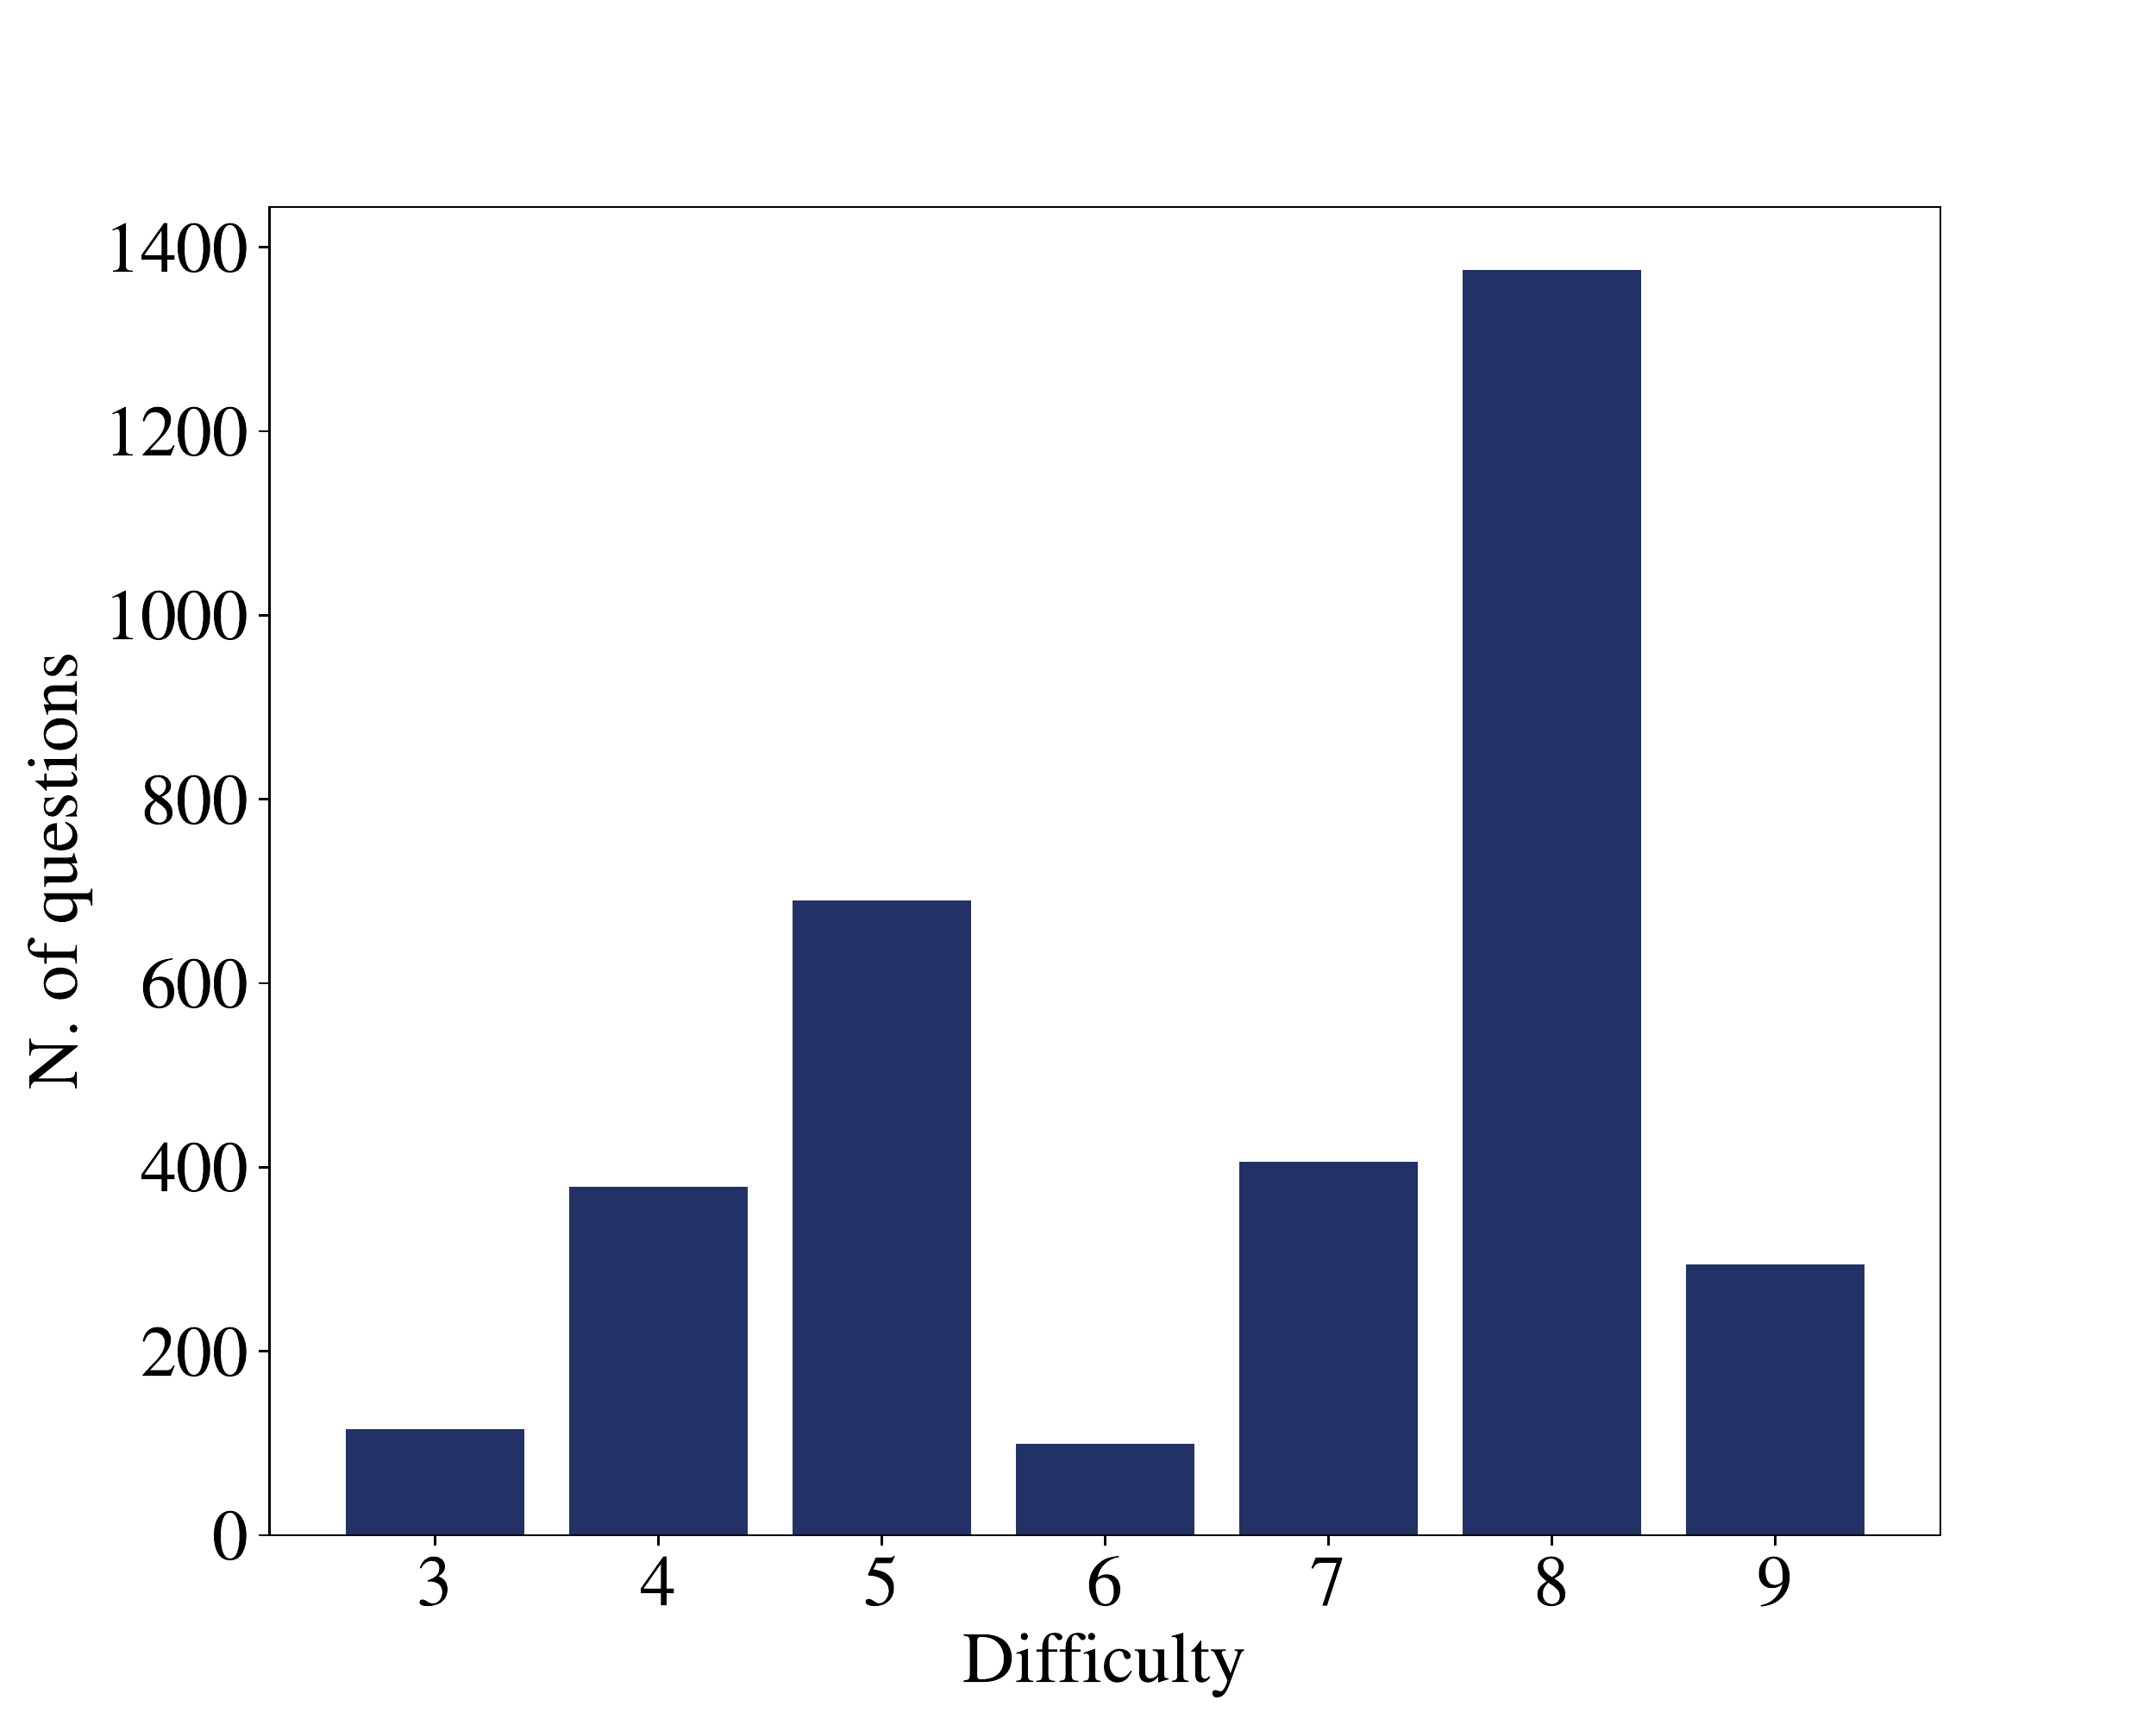}
\caption{Train.}
\label{fig:diff_distr_arc_train}
\end{subfigure}
\begin{subfigure}{0.40\textwidth}
\centering
\includegraphics[width=\textwidth]{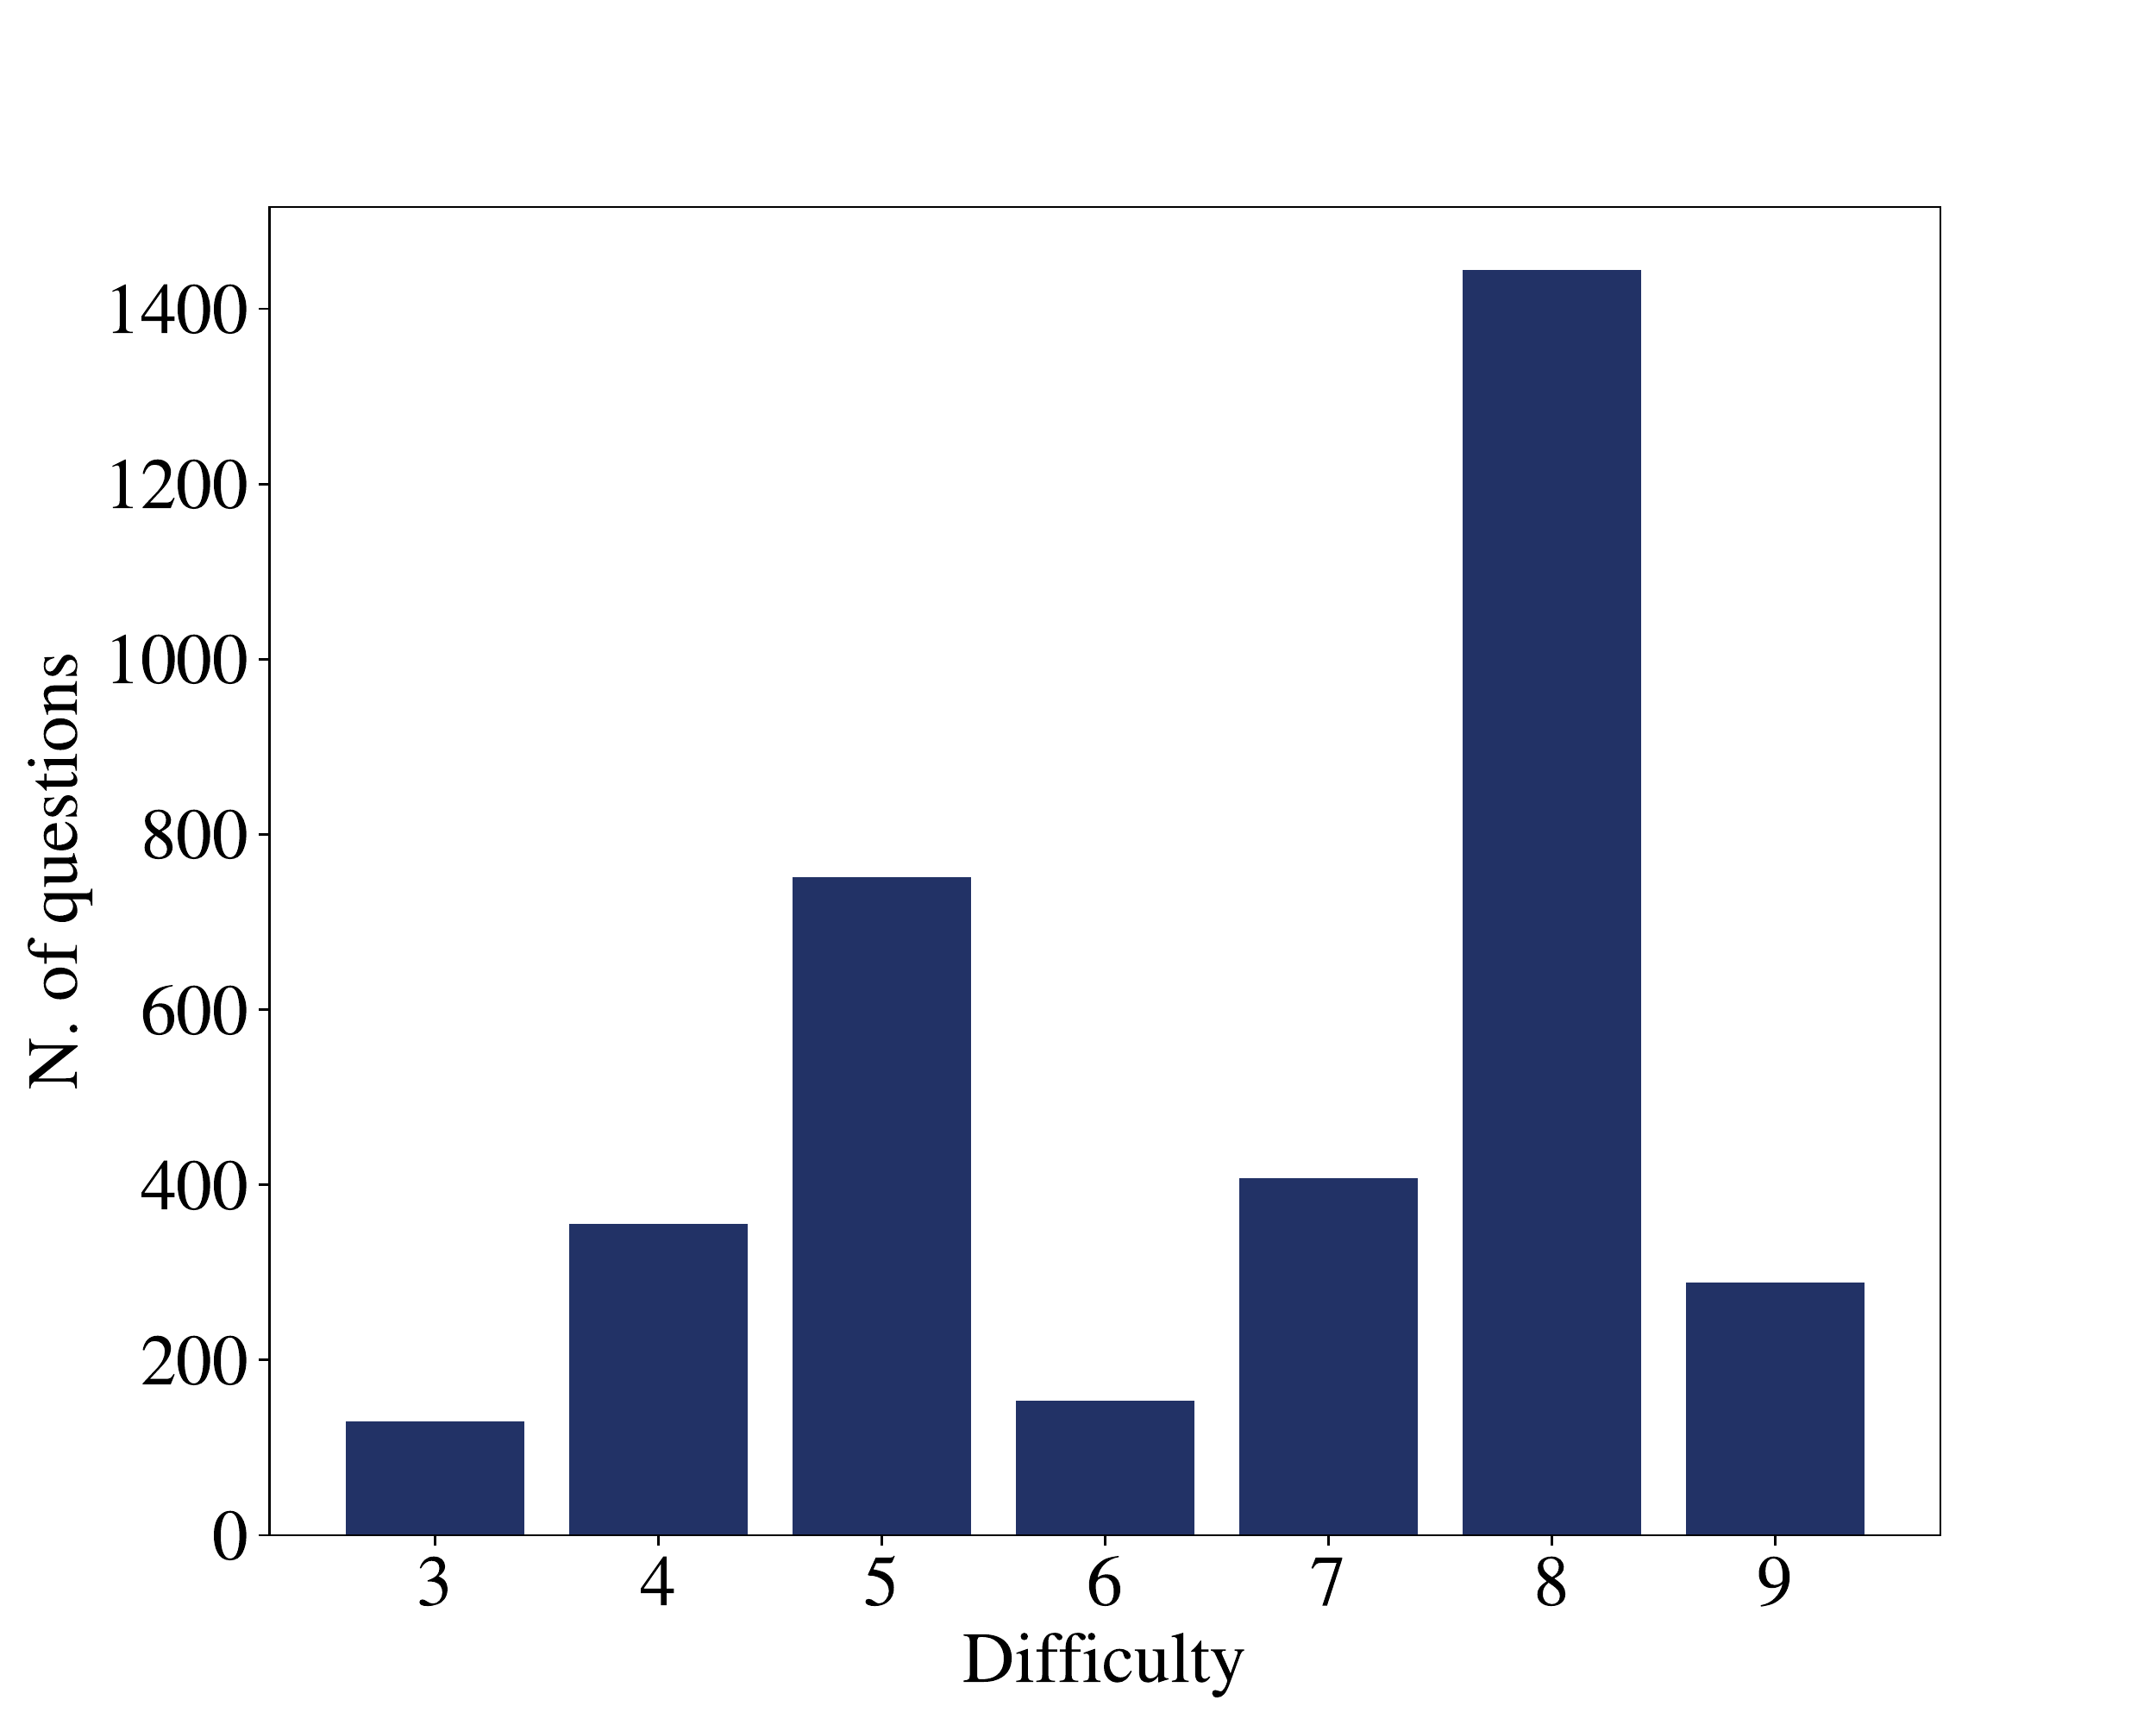}
\caption{Test.}
\label{fig:diff_distr_arc_test}
\end{subfigure}
\caption{Question distribution by difficulty in \arc{}.}
\label{fig:diff_distr_arc}
\end{figure}

Figure \ref{fig:app:diff_distr_arc_balanced_train} shows the distributions of questions per difficulty level in the train split of \arc{} after the subsampling to partially balance the different labels.
We only sub-sample the training set, thus changing the distribution of the train with respect to the test set, but it is not a problem for this application.
Indeed, we ideally want the models to have the same accuracy across different difficulty levels, and not simply obtain the best results from an evaluation metric point of view.

\begin{figure}
\centering
\includegraphics[width=.5\textwidth]{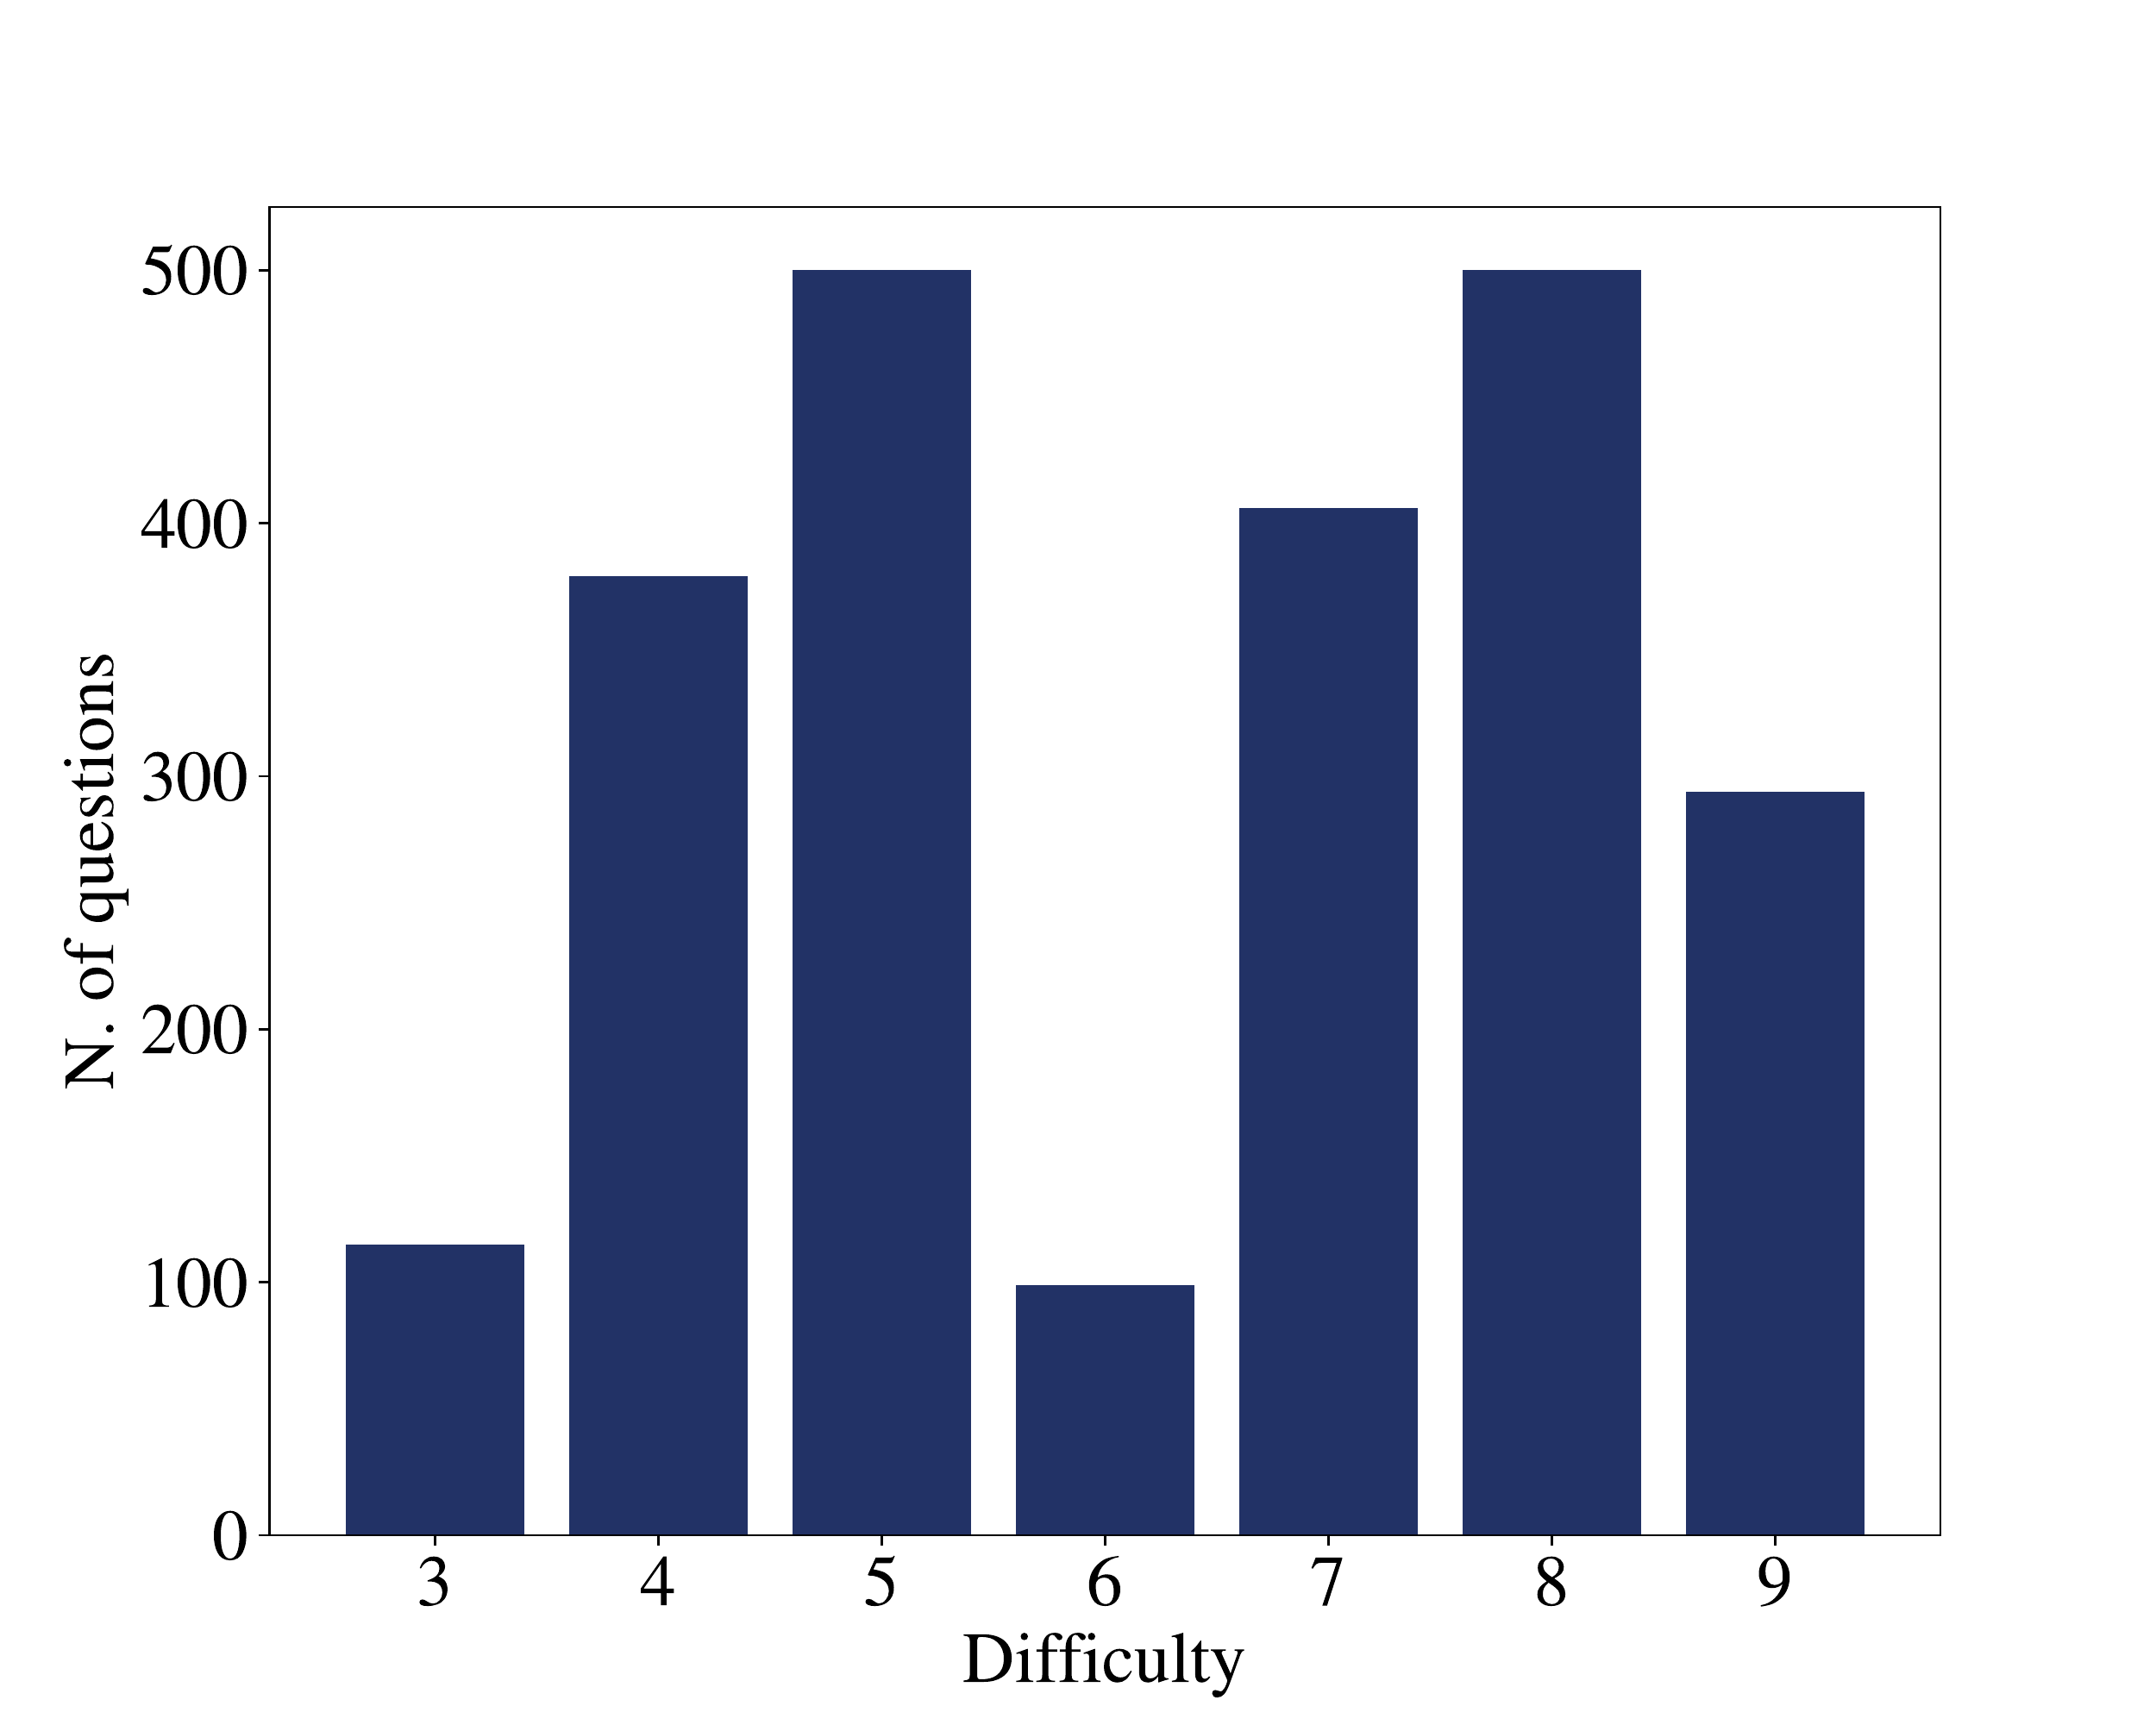}
\caption{Question distribution by difficulty in the \arc{} training set, after subsampling.}
\label{fig:app:diff_distr_arc_balanced_train}
\end{figure}

\subsection{\am{}}
%TODO ? something else? Such as stats
The text of the questions in \am{} and the interaction data for pretesting is available at \url{https://sites.google.com/site/assistmentsdata/}.

Figure \ref{fig:diff_distr_am} shows the distribution of questions by difficulty in \am{} in the train and test splits.
Differently from the two previous datasets, in this case the difficulty is continuous, and it follows a Gaussian-like distribution with mean close to 0.
The small ``peaks'' visible for difficulty of $-5$ and $+5$ are the questions which are correctly and wrongly answered by all the students used for pretesting.

\begin{figure}
\centering
\begin{subfigure}{0.40\textwidth}
\centering
\includegraphics[width=\textwidth]{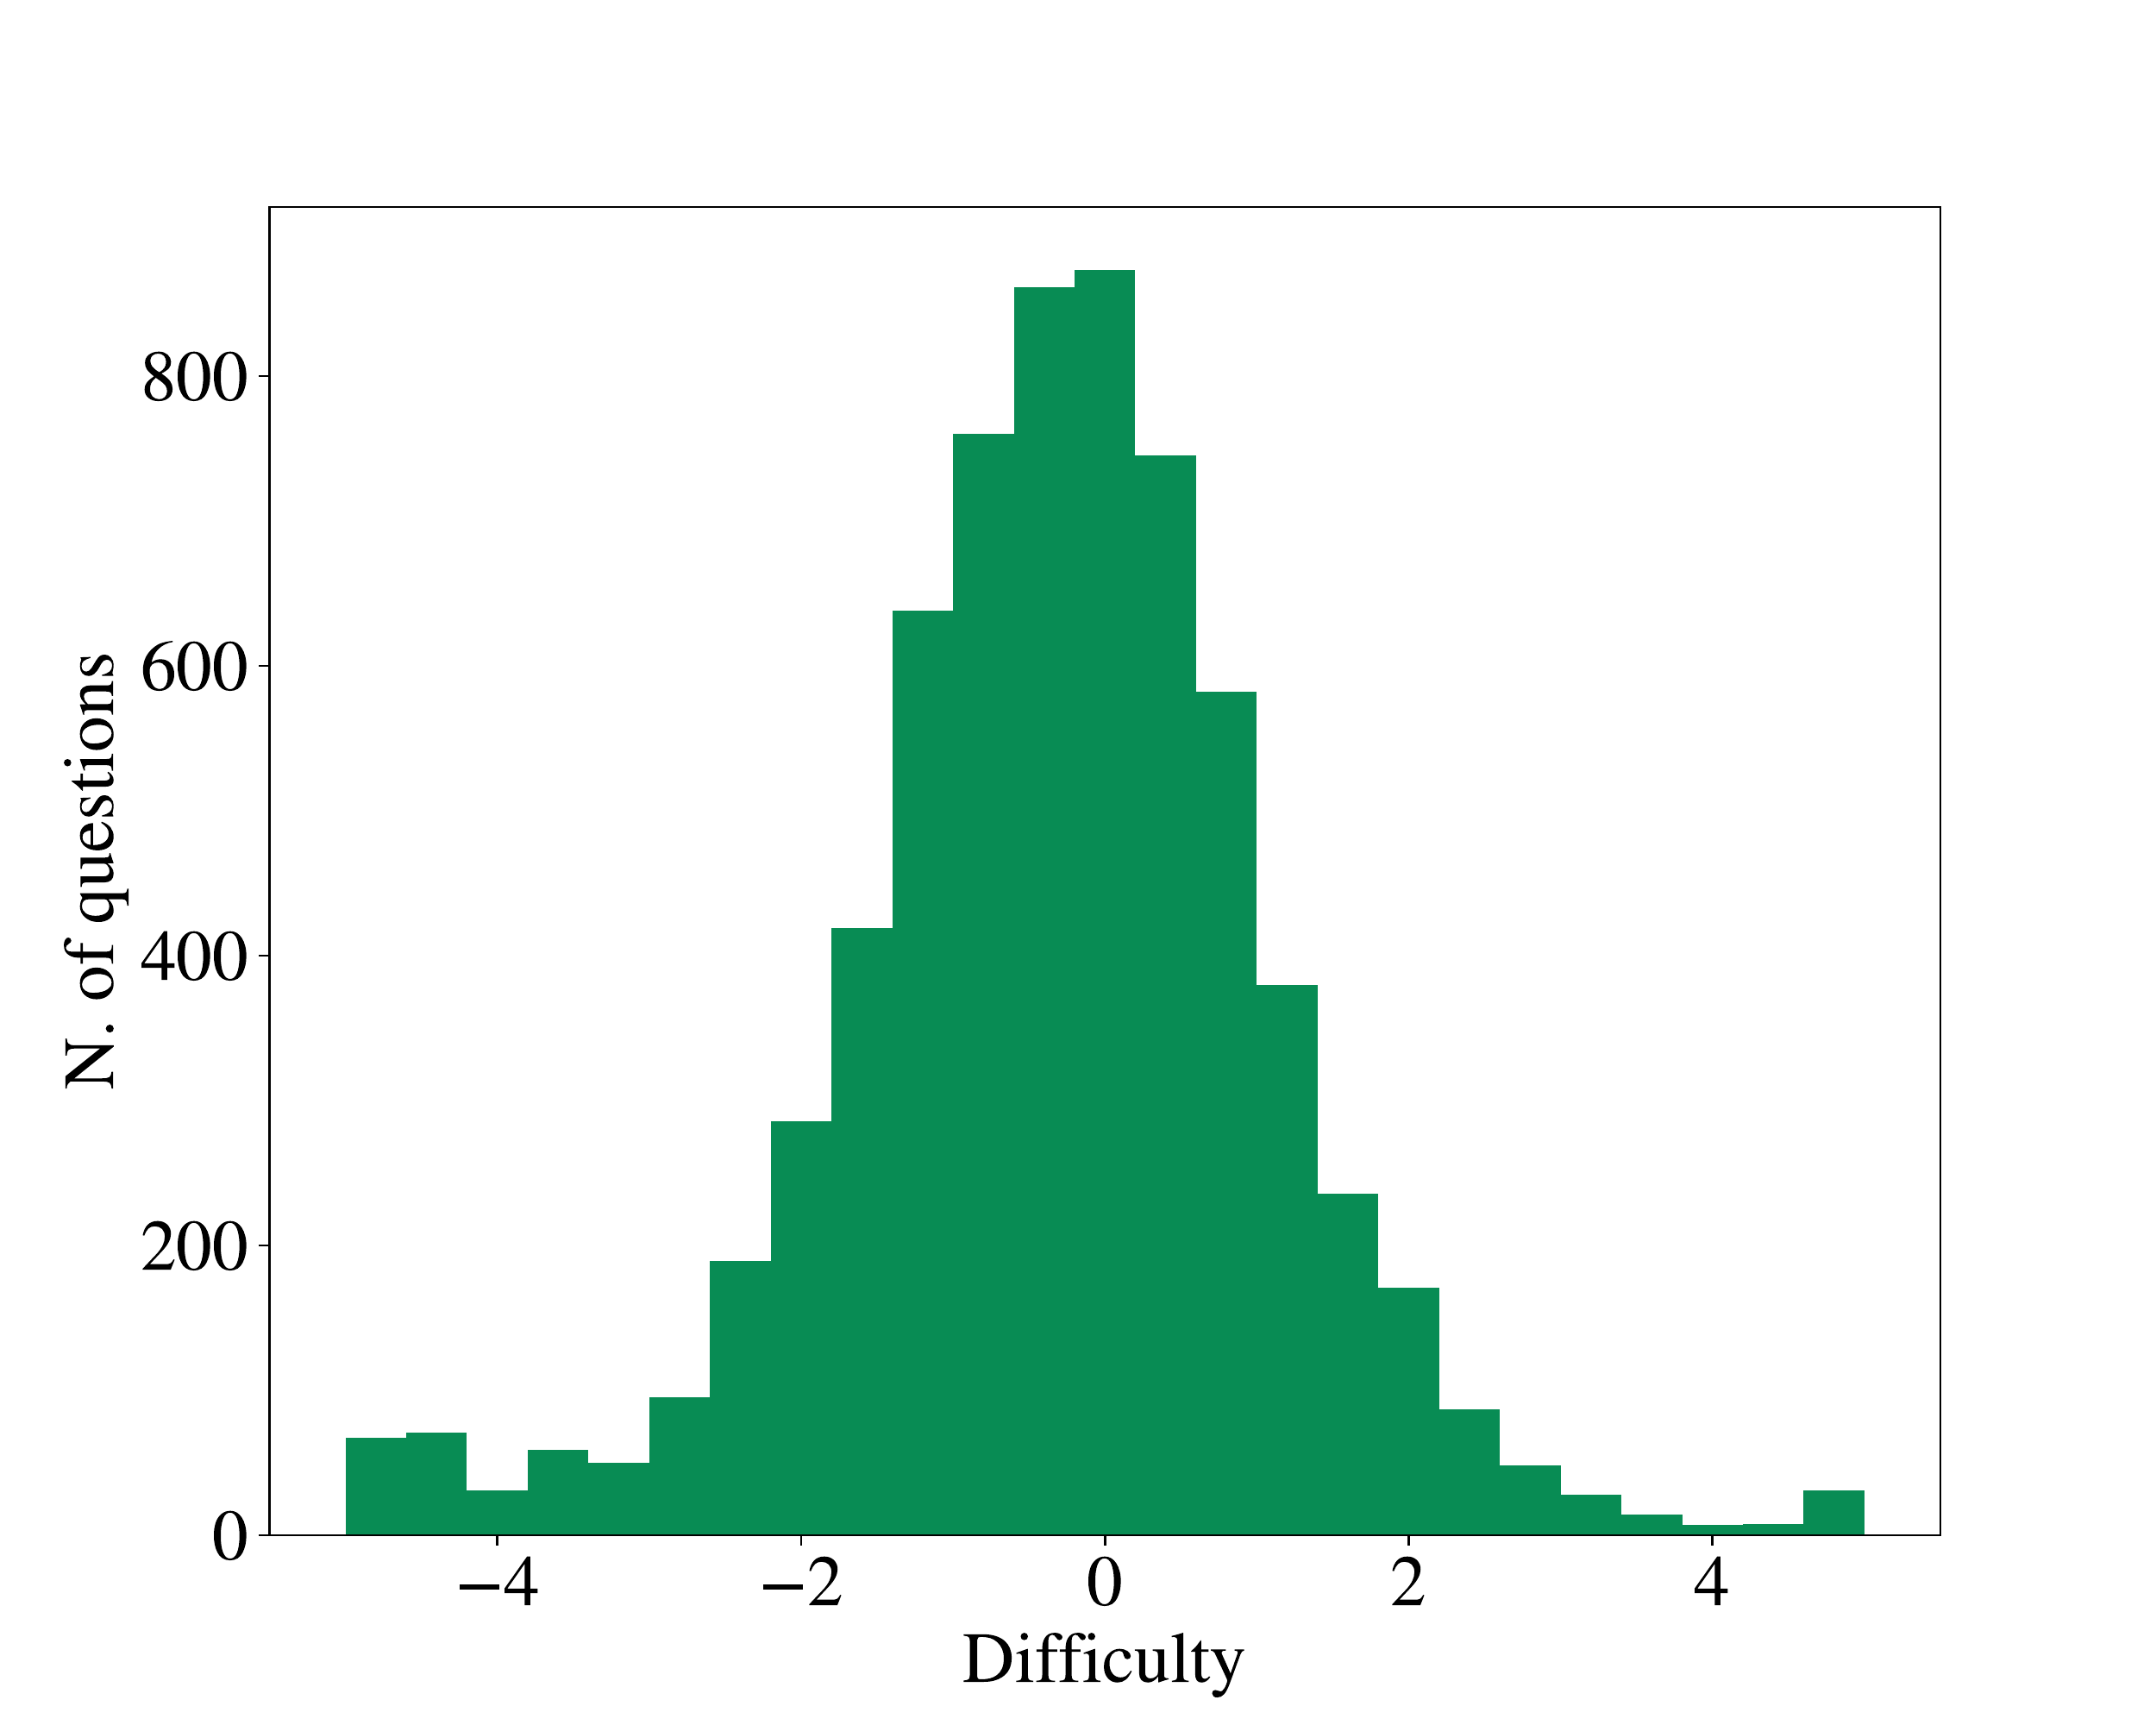}
\caption{Train.}
\label{fig:diff_distr_am_train}
\end{subfigure}
\begin{subfigure}{0.40\textwidth}
\centering
\includegraphics[width=\textwidth]{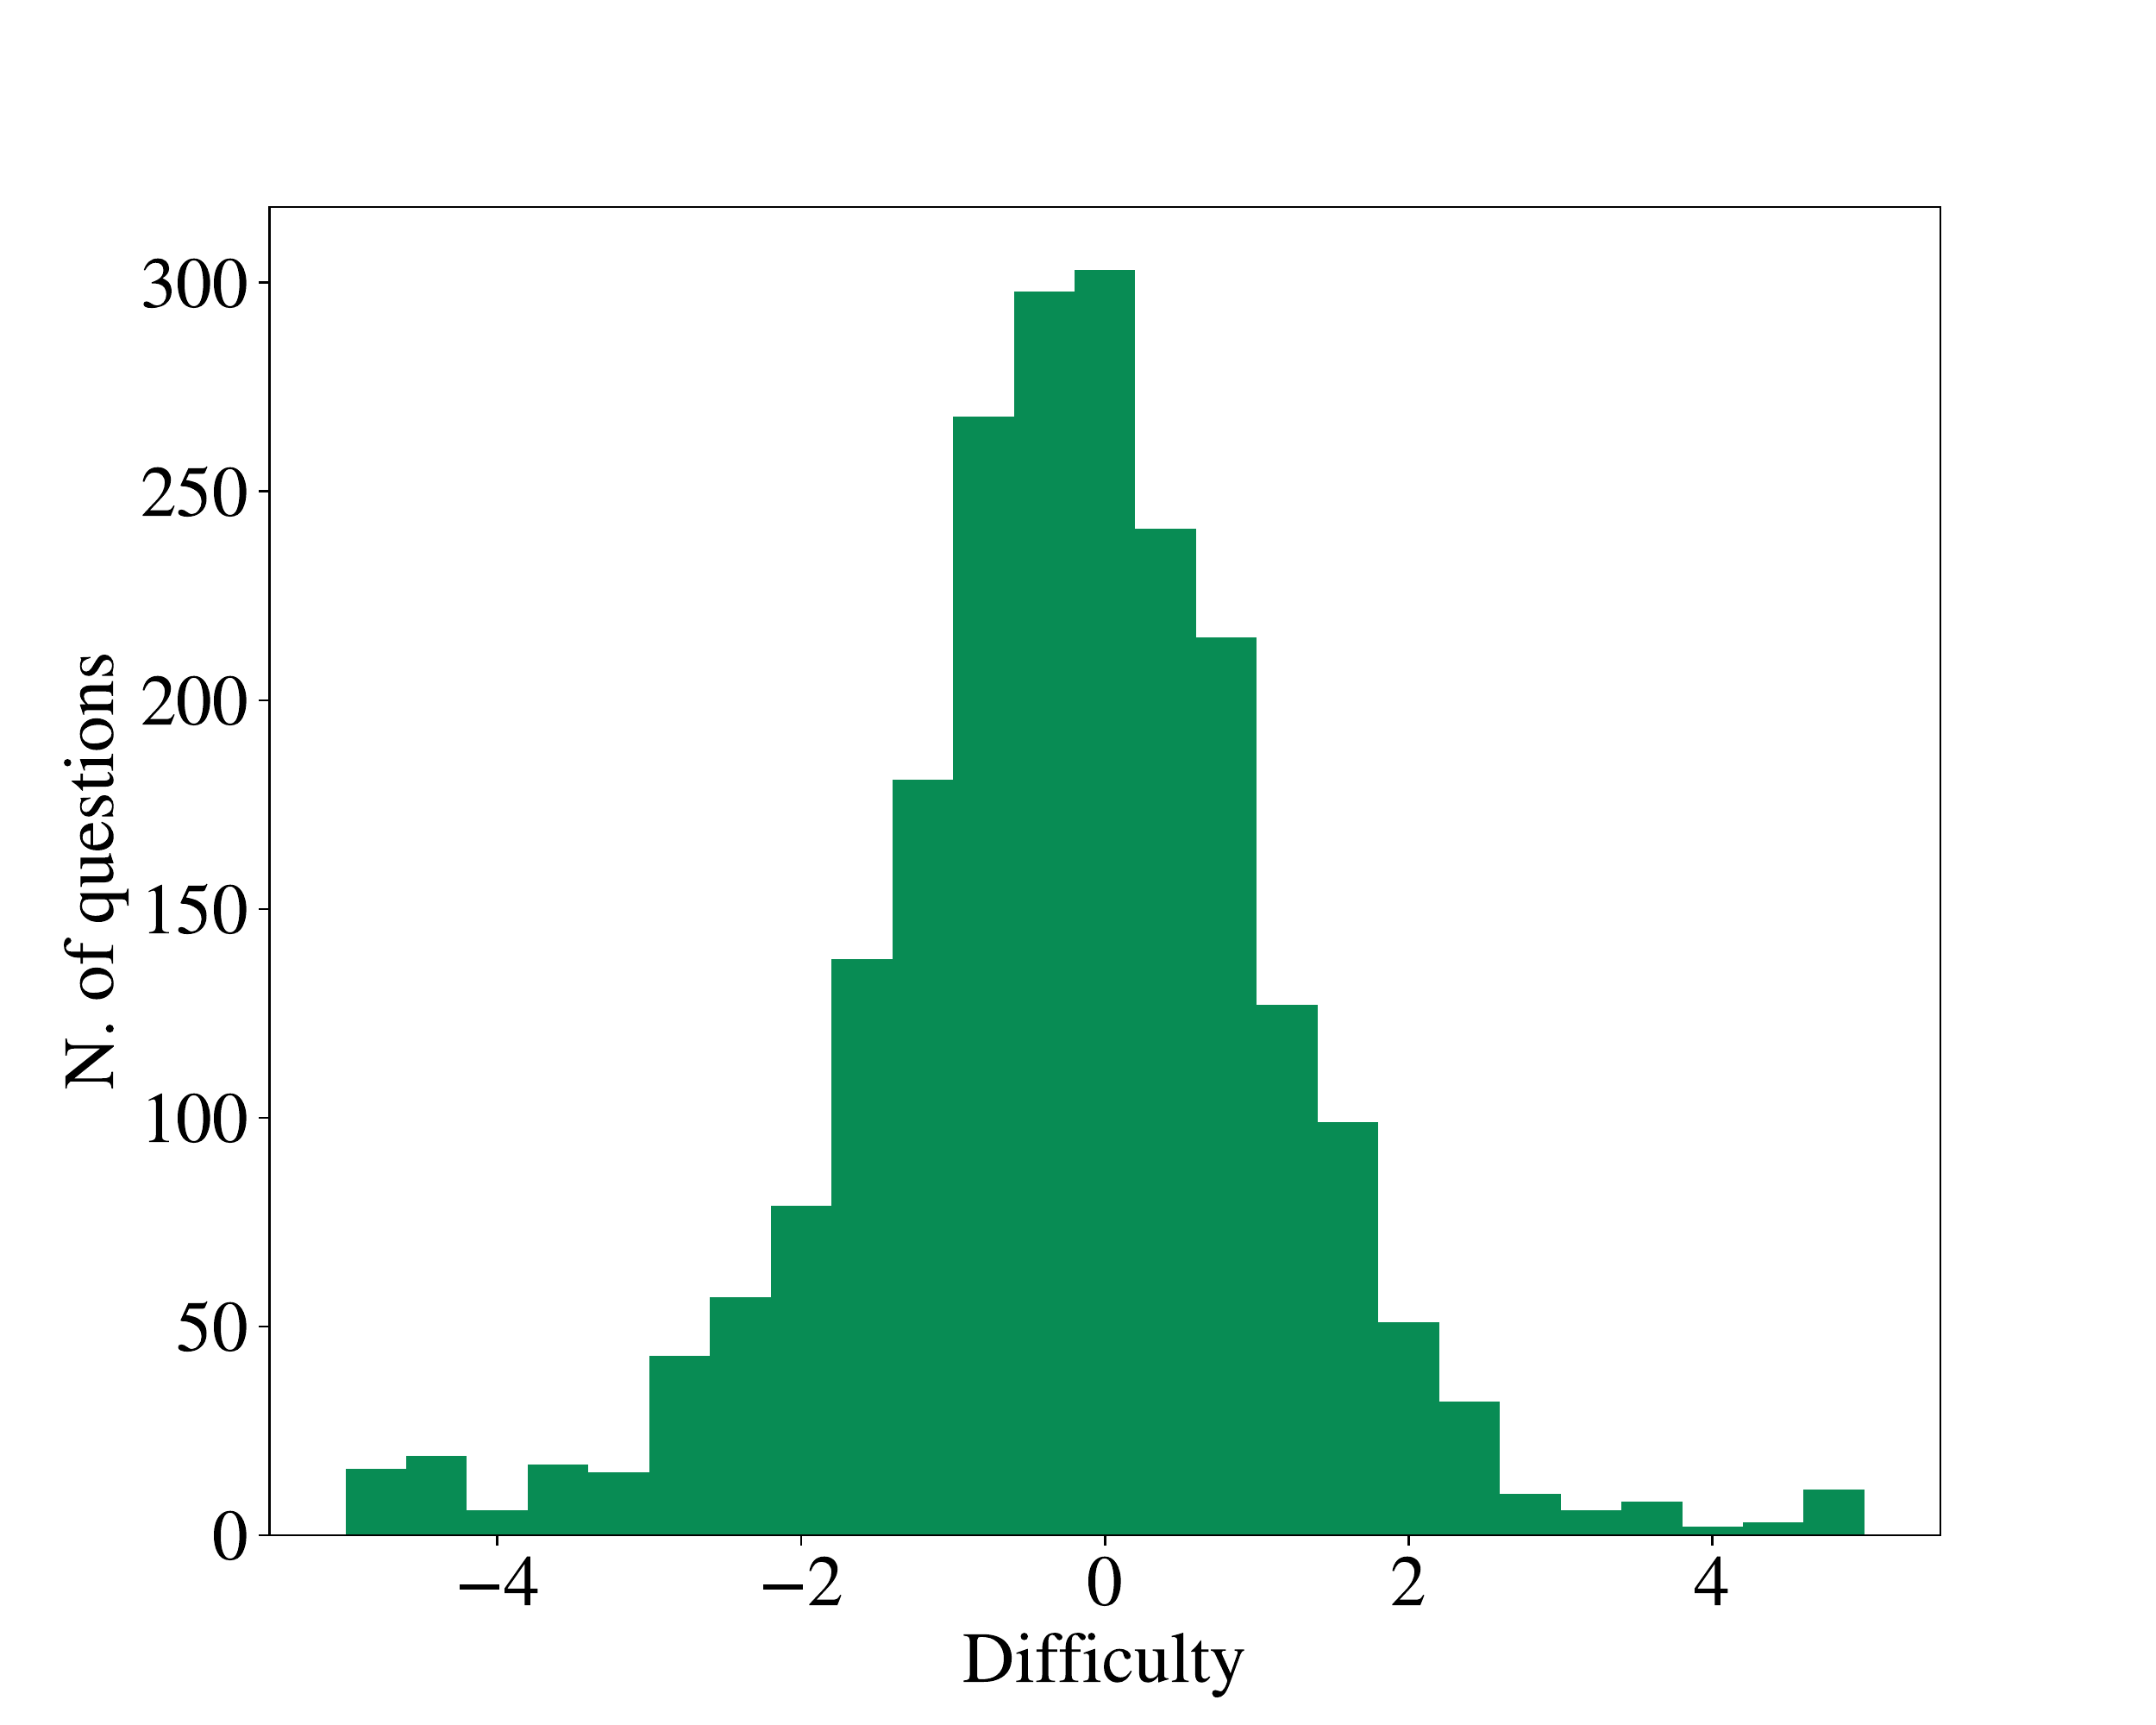}
\caption{Test.}
\label{fig:diff_distr_am_test}
\end{subfigure}
\caption{Question distribution by difficulty in \am{}.}
\label{fig:diff_distr_am}
\end{figure}
