# Supplementary material for: A quantitative study of NLP approaches to question difficulty estimation
Source: arXiv:2305.10236 source file (2023-05-17)
Supplement: Supplementary file 2 [file appendix_models.tex]

\section{Models}

\subsection{Linguistic Features}\label{app:sec:ling}
The complete list of linguistic features used in this study is the following.
\begin{itemize}
\item number of words in the question, 
\item number of words in the correct answer, 
\item average number of words in the distractors, 
\item numer of sentences in the question,
\item number of sentences in the correct answer,
\item average number of sentences in the distractors,
\item average word length in the question,
\item ratio between the length of the question and the length of the answer,
\item ratio between the length of the question and the length of the distractors,
\item number of characters in the question,
\item average sentence length in the question,
\item average number of nouns per sentence in the question,
\item average number of verbs per sentence in the question,
\item number of long words (seven characters or more) in the question,
\item number of short words in the question,
\item average number of long words per sentence in the question,
\item average number of short words per sentence in the question.
\end{itemize}

%\subsection{Readability Features}\label{app:sec:read}
%Flesch Reading Ease \cite{flesch1948new}:

%Flesch-Kincaid Grade Level \cite{kincaid1975derivation}: 

%ARI \cite{senter1967automated}:

%Gunning FOG Index \cite{gunning1952technique}: 

%Coleman-Liau Index \cite{coleman1965understanding}:

%Linsear Write Formula \cite{klare1974assessing}:

%Dale-Chall Readability Score \cite{dale1948formula}:
