# Supplementary material for: A quantitative study of NLP approaches to question difficulty estimation
Source: arXiv:2305.10236 source file (2023-05-17)
Supplement: Supplementary file 5 [file appendix_results.tex]

\section{Results}

\subsection{Variation in performance depending on training dataset size}\label{app:sec:variation_performance}
Figure \ref{fig:app:r2_per_size} plots, for different models, how the R2 metric on the test set vary depending on the training size. 
The observations are similar to the ones made in Section \ref{sec:results}: the metric generally improves for larger training sizes, with the only exception of BERT \qa{} and TF-IDF \qc{} for \raceeightk{}.
As observed in the main results section, even when trained on the smaller \racefourk{} the Transformers perform better than or similar to the other models trained on the whole \race{}.

\begin{figure}
\centering
\includegraphics[width=.5\textwidth]{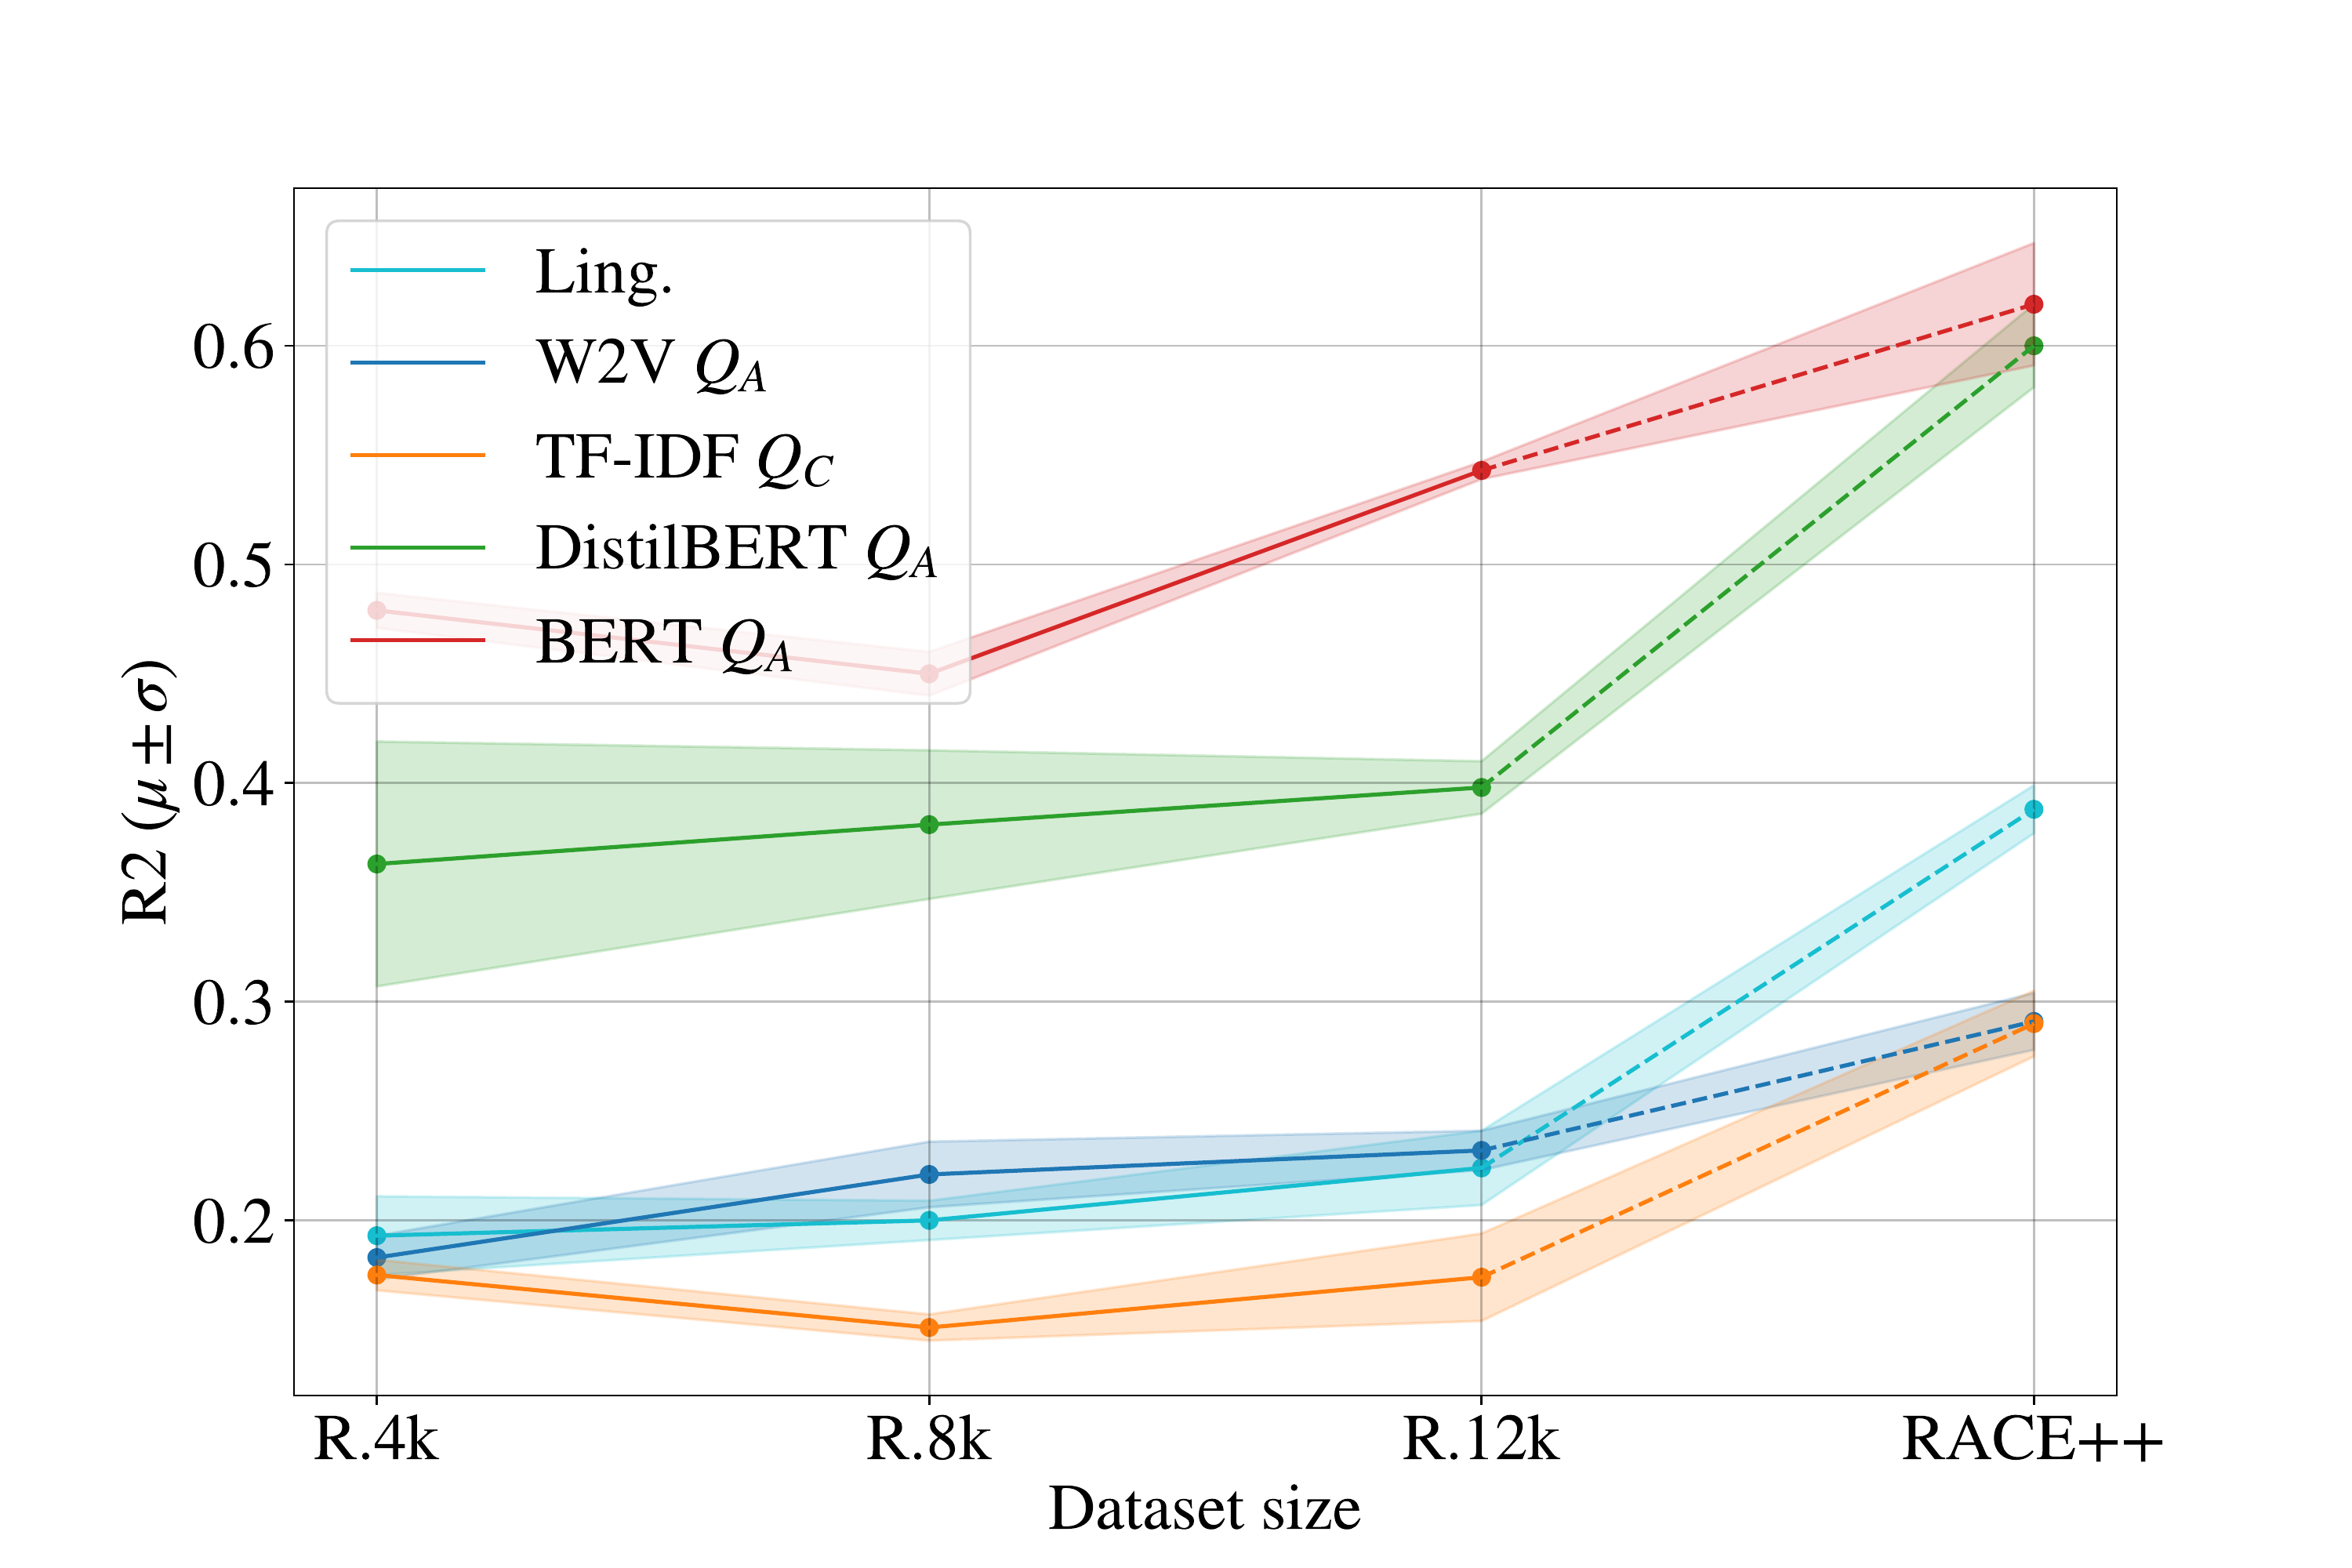}
\caption{R2.}
\label{fig:app:r2_per_size}
\end{figure}
